# Supplementary material for: Distributed quantum sensing with multi-mode $N00N$ states
Source: arXiv:2508.02070 ancillary file (2025-08-04)
Supplement: Supplementary file 1 [file DistributedN00N_Supplementary_v8.pdf]

# Supplemental Material for: Distributed quantum sensing with multi-mode $N00N$ states

Dong-Hyun Kim,[1,2,*] Seongjin Hong,[2,*] Yong-Su Kim,[1,3] Kyunghwan Oh,[2] Su-Yong Lee,[4,5] Changhyoup Lee,[6] and Hyang-Tag Lim[1,3,†]

[1] *Center for Quantum Technology, Korea Institute of Science and Technology (KIST), Seoul, 02792, Korea*
[2] *Department of Physics, Yonsei University, Seoul 03722, Korea*
[3] *Division of Quantum Information, KIST School, Korea University of Science and Technology, Seoul 02792, Korea*
[4] *Emerging Science and Technology Directorate, Agency for Defense Development, Daejeon 34186, Korea*
[5] *Weapon Systems Engineering, ADD School, University of Science and Technology, Daejeon, 34060, Korea*
[6] *Korea Research Institute of Standards and Science, Daejeon 34113, Korea*

[*] These authors contributed equally
[†] hyangtag.lim@kist.re.kr

## I. THEORETICAL ANALYSIS OF THE SENSITIVITY BOUND

We consider probe states such as multi-mode $N00N$ states [1], separable $N00N$ states, product states of multiple coherent states as shown in Supplemental Figure (1), and mode- and particle-entangled (MePe) states [2, 3].

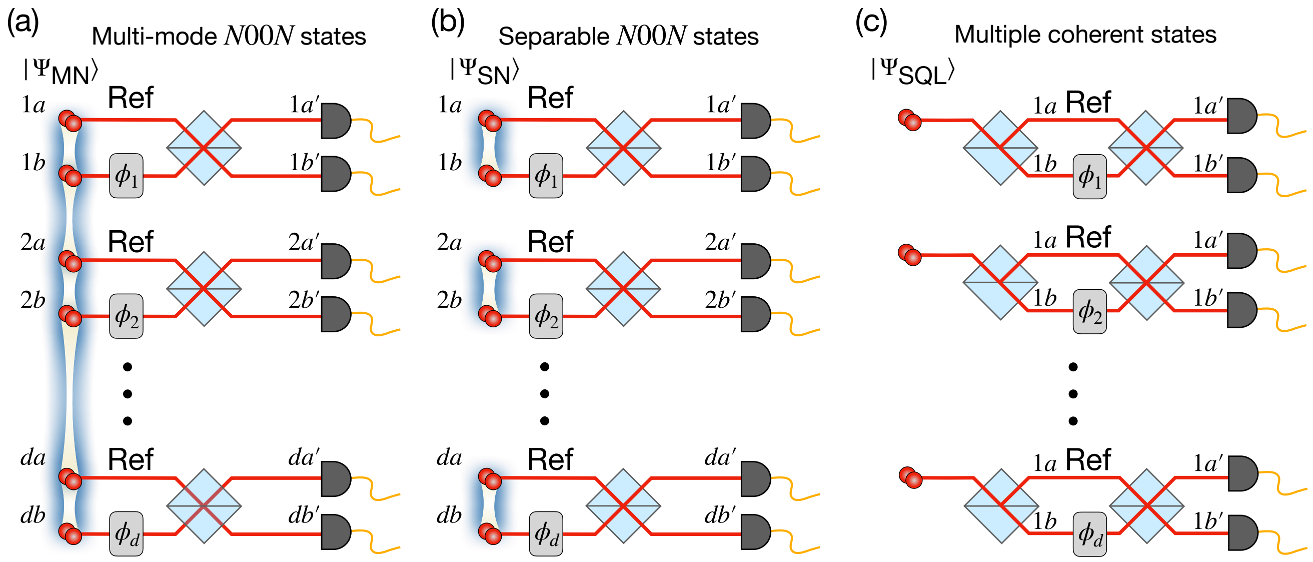


Supplemental Figure 1. **Scheme for distributed quantum sensing with considered probe states.** The probe states are distributed among $d$ nodes for estimating the spatially distributed phases. After phase encoding in each $b$ mode, the probe states in mode $a$ and $b$ enter into 2×2 beam splitters for local measurement. Estimation process for multi-mode $N00N$ states (a), separable $N00N$ states (b), and product states of multiple coherent states (c).

### A. Multi-mode $N00N$ states

First, the unitary matrix for encoding phases in the probe state is given by

$$\hat{U}(\phi) = \bigotimes_{j=1}^{d} \hat{U}(\phi_j) = \begin{pmatrix} 1 & 0 & 0 & 0 & \cdots & 0 \\ 0 & e^{i\phi_1} & 0 & 0 & \cdots & 0 \\ 0 & 0 & 1 & 0 & \cdots & 0 \\ 0 & 0 & 0 & e^{i\phi_2} & \cdots & 0 \\ \vdots & \vdots & \vdots & \vdots & \ddots & \vdots \\ 0 & 0 & 0 & 0 & 0 & e^{i\phi_d} \end{pmatrix}, \tag{1}$$

where $j$ denotes the node, and

$$\hat{U}(\phi_j) = \begin{pmatrix} 1 & 0 \\ 0 & e^{i\phi_j} \end{pmatrix}. \tag{2}$$

The multi-mode $N00N$ states after the local phase evolution, as shown in Supplemental Figure 1(a), can be written as

$$\begin{aligned} \hat{U}(\boldsymbol{\phi})|\Psi_{\mathrm{MN}}\rangle = \frac{1}{\sqrt{2d}}(&|N0\rangle_1|00\rangle_2\ldots|00\rangle_{d-1}|00\rangle_d + e^{iN\phi_1}|0N\rangle_1|00\rangle_2\ldots|00\rangle_{d-1}|00\rangle_d \\ &+ |00\rangle_1|N0\rangle_2\ldots|00\rangle_{d-1}|00\rangle_d + e^{iN\phi_2}|00\rangle_1|0N\rangle_2\ldots|00\rangle_{d-1}|00\rangle_d + \cdots \\ &+ |00\rangle_1|00\rangle_2\ldots|00\rangle_{d-1}|N0\rangle_d + e^{iN\phi_d}|00\rangle_1|00\rangle_2\ldots|00\rangle_{d-1}|0N\rangle_d), \end{aligned} \tag{3}$$

where $N$ represents the number of photons.

Using elements of the quantum Fisher information matrix (QFIM), $F_{\mathrm{Q}(j,k)} = 4\mathrm{Re}[\langle\partial_{\phi_j}\Psi|\partial_{\phi_k}\Psi\rangle - \langle\partial_{\phi_j}\Psi|\Psi\rangle\langle\Psi|\partial_{\phi_k}\Psi\rangle]$, we can construct the QFIM of $|\Psi_{\mathrm{MN}}\rangle$, corresponding to Eq. (4) of the main text, as follows:

$$\mathbf{F}_{\mathrm{Q}}^{\mathrm{MN}} = \begin{pmatrix} (2d-1)N^2/d^2 & -(N/d)^2 & \cdots & -(N/d)^2 \\ -(N/d)^2 & & & \vdots \\ \vdots & & \ddots & -(N/d)^2 \\ -(N/d)^2 & \cdots & -(N/d)^2 & (2d-1)N^2/d^2 \end{pmatrix}. \tag{4}$$

Using the Eq. (1) of the Main text, the sensitivity bound of $|\Psi_{\mathrm{MN}}\rangle$ can be obtained as $1/N^2$, achieving the Heisenberg scaling (HS) of $1/N^2$, similar to the previously proposed MePe states [2, 3]. To calculate the classical Fisher information matrix (CFIM) of $|\Psi_{\mathrm{MN}}\rangle$, we consider the local measurements consisting of $2\times2$ beam splitter (BS) and photon number resolving detector (PNRD). The elements of the CFIM are given by $F_{\mathrm{C}(j,k)} = \sum_l (1/P_l)(\partial P_l/\partial\phi_j)(\partial P_l/\partial\phi_k)$. The unitary matrix for local measurements using $2\times2$ BS is given by

$$\hat{U}_{\mathrm{BS}}^{\otimes d} = \frac{1}{\sqrt{2}}\begin{pmatrix} 1 & i \\ i & 1 \end{pmatrix}^{\otimes d}. \tag{5}$$

After passing through the phase shifts and $2\times2$ BS, the final state can be written as:

$$\begin{aligned} |\Psi_{\mathrm{out}}\rangle &= \hat{U}_{\mathrm{BS}}^{\otimes d}\hat{U}(\phi)|\Psi_{\mathrm{MN}}\rangle \\ &= \sum_j^d [[\frac{1}{\sqrt{2d}}\hat{U}_{\mathrm{BS}}^{\otimes d}\hat{U}(\phi_j)(|N0\rangle_j + |0N\rangle_j)] \bigotimes_{j\neq k}^d |00\rangle_k)] \\ &= \sum_j^d (\sum_m c_{m,j}|\psi\rangle_{m,j}) \bigotimes \sum_{j\neq k}^d |00\rangle_k, \end{aligned} \tag{6}$$

where $c_{m,j}$ is the amplitude of the two-mode $N00N$ states at $j$ node after passing phase encodnig and the $2\times2$ BS. Using Supplemental Eq. (6), we can obtain the detection probability for $|\Psi_{\mathrm{MN}}\rangle$ as follows:

$$P_l = \frac{|c_{m,j}|^2}{\sum_j^d\sum_m |c_{m,j}|^2} = \frac{|c_l|^2}{\sum_l |c_l|^2}. \tag{7}$$

Then, we calculate the CFIM of $|\Psi_{\mathrm{MN}}\rangle$ using Supplemental Eq. (7) as follows:

$$\mathbf{F}_{\mathrm{C}}^{\mathrm{MN}} = \begin{pmatrix} N^2/d & 0 & \cdots & 0 \\ 0 & & & \vdots \\ \vdots & & \ddots & 0 \\ 0 & \cdots & 0 & N^2/d \end{pmatrix}. \tag{8}$$

One can find that using the local measurements with $|\Psi_{\mathrm{MN}}\rangle$ can achieve the HS of $1/N^2$. Thus, the sensitivity bound for $|\Psi_{\mathrm{MN}}\rangle$ can be written as

$$\Delta^2\phi_{\mathrm{MN}} \geq \frac{1}{N^2}. \tag{9}$$

It is also notable that the QCRB of mode-entangled states can be saturated by local measurements consisting of BS and PNRD for estimating $\phi$, even though $\mathbf{F}_{\mathrm{C}}^{\mathrm{MN}}$ has all zero off-diagonal elements that describe correlations between two different nodes.

### B. Separable two-mode *N00N* states

Then, we consider the separable two-mode $N00N$ states as shown in Supplemental Figure 1(b). $|\Psi_{\mathrm{SN}}\rangle$ to compare with other probe states. $|\Psi_{\mathrm{SN}}\rangle$ is given by

$$|\Psi_{\mathrm{SN}}\rangle = \bigotimes_{j=1}^d (\frac{1}{\sqrt{2}}(|\frac{N}{d}0\rangle_j + |0\frac{N}{d}\rangle_j)), \tag{10}$$

$$\xrightarrow{\text{Phase Encoding } \phi} \hat{U}(\phi)|\Psi_{\mathrm{SN}}\rangle = \bigotimes_{j=1}^{d} (\frac{1}{\sqrt{2}}(|\frac{N}{d}0\rangle_j + e^{i(N/d)\phi_j}|0\frac{N}{d}\rangle_j)). \tag{11}$$

Then, we calculate the QFIM using Supplemental Eq. (11). It is known that the CRB can saturate the QCRB with N00N states in Ref. [4]. The QFIM for $|\Psi_{\mathrm{SN}}\rangle$ is obtained as follows:

$$\mathbf{F}_{\mathrm{Q}}^{\mathrm{SN}} = \mathbf{F}_{\mathrm{C}}^{\mathrm{SN}} = \begin{pmatrix} (N/d)^2 & 0 & \cdots & 0 \\ 0 & & & \vdots \\ \vdots & & \ddots & 0 \\ 0 & \cdots & 0 & (N/d)^2 \end{pmatrix}. \tag{12}$$

We also obtain the CFIM of $|\Psi_{\mathrm{SN}}\rangle$ with local measurements, which results in the same matrix as the QFIM, i.e., $\mathbf{F}_{\mathrm{Q}}^{\mathrm{SN}} = \mathbf{F}_{\mathrm{C}}^{\mathrm{SN}}$. Thus, the sensitivity bound for $|\Psi_{\mathrm{SN}}\rangle$ can be obtained as follows:

$$\Delta^2\phi_{\mathrm{SN}} \geq \frac{d}{N^2}. \tag{13}$$

### C. Standard quantum limit

To derive the standard quantum limit (SQL), which is achievable using classical resources, we consider product states of multiple coherent states as the classical state. $|\Psi_{\mathrm{SQL}}\rangle$, as shown in Supplemental Figure 1(c), is given by

$$|\Psi_{\mathrm{SQL}}\rangle = \bigotimes_{j=1}^{d} |\alpha_j\rangle, \tag{14}$$

where $|\alpha_j|^2 = N/d$. It is well known that coherent states give the sensitivity of $1/|\alpha|^2$ for estimating a single parameter. In distributed quantum sensing, for estimating the global function of unknown phases, one can readily obtain $\Delta\phi^2_{\mathrm{SQL}} = 1/N$ using error propagation. The sensitivity bound for $|\Psi_{\mathrm{SQL}}\rangle$ is given by

$$\Delta^2\phi_{\mathrm{SQL}} \geq \frac{1}{N}. \tag{15}$$

### D. Mode- and particle-entangled states

We now consider MePe states, $|\Psi_{\mathrm{MePe}}\rangle$, which achieve the HS of $1/N^2$. We directly adopt the form of $|\Psi_{\mathrm{MePe}}\rangle$ from Ref. [5]:

$$|\Psi_{\mathrm{MePe}}\rangle = \frac{1}{\sqrt{2}}(\otimes_{j=1}^{d}|(\frac{N}{d})_j, \lambda_j^+\rangle^{\otimes d} + |(\frac{N}{d})_j, \lambda_j^-\rangle^{\otimes d}), \tag{16}$$

$$\xrightarrow{\text{Phase Encoding } \phi} U(\phi)|\Psi_{\mathrm{MePe}}\rangle = \frac{1}{\sqrt{2}}(\otimes_{j=1}^{d}|(\frac{N}{d})_j, \lambda_j^+\rangle^{\otimes d} + e^{\sum_{j=1}^{d} i(N/d)\phi_j}|(\frac{N}{d})_j, \lambda_j^-\rangle^{\otimes d}) \tag{17}$$

where $|\lambda_j^{\pm}\rangle$ denotes eigenvectors at each node, with superscripts $\pm$ representing the eigenvalues. Here, we consider polarization-entangled states proposed in Ref. [2, 3], with $\lambda_j^{\pm} = \pm 1$. Here we focus on the QCRB and note that the CRB can also be saturated with MePe states, as shown in Ref. [2, 3].

We calculate the QFIM for $|\Psi_{\mathrm{MePe}}\rangle$ as follows:

$$\mathbf{F}_{\mathrm{Q}}^{\mathrm{MePe}} = \begin{pmatrix} (N/d)^2 & \cdots & (N/d)^2 \\ \vdots & \ddots & \vdots \\ (N/d)^2 & \cdots & (N/d)^2 \end{pmatrix}. \tag{18}$$

However, the QFIM of $|\Psi_{\mathrm{MePe}}\rangle$ is singular, thus we use a weak form of the QCRB to obtain the sensitivity bound [5]. The weak form of the QCRB are given by

$$\Delta^2\phi_{\mathrm{MePe}} \geq \frac{(\boldsymbol{\nu}^T\boldsymbol{\nu})^2}{\mu\boldsymbol{\nu}^T\mathbf{F}_{\mathrm{Q}}^{\mathrm{MePe}}\boldsymbol{\nu}}. \tag{19}$$

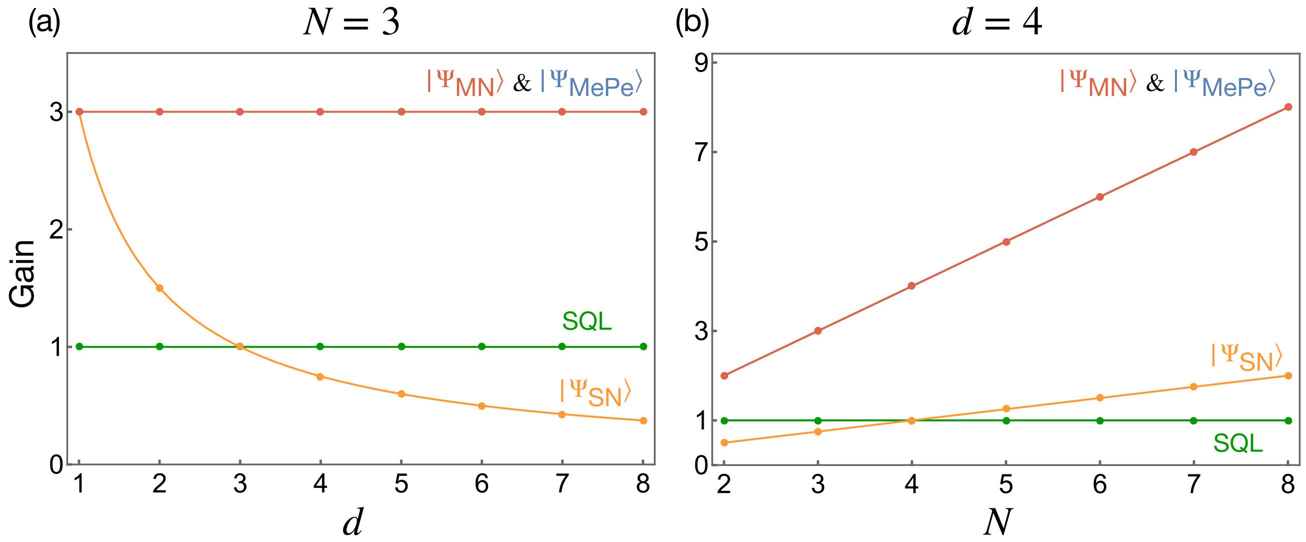


Supplemental Figure 2. **Gain in sensitivity for considering the probe states.** (a) Gain in sensitivity compared with the probe states as a function of the number of nodes, $d$ with $N=3$. (b) Gain in sensitivity for the probe states as a function of the number of photons, $N$ with $d=4$.

Using Supplemental Eqs. (18) and (19), we can derive the sensitivity bound for $|\Psi_{\text{MePe}}\rangle$ as follows:

$$\Delta^2\phi_{\text{MePe}} \geq \frac{1}{N^2}. \tag{20}$$

This confirms that the sensitivity bound for $|\Psi_{\text{MePe}}\rangle$ achieves the HS, providing a precision limit of $1/N^2$.

### E. Gain

The gain in sensitivity of the probe states can be obtained by $G = \Delta^2\phi_{\text{SQL}}/\Delta^2\phi$, where $G$ for $|\Psi_{\text{SQL}}\rangle$ is 1. Using the sensitivity bound for the probe states derived above, we calculated the gain as a function of the number of photons and phases, as shown in Supplemental Figure 2. Note that $|\Psi_{\text{SN}}\rangle$ can be practically realized when $N/d$ is an integer. The obtained gain for the considered probe states is presented in Table I of the main text. $|\Psi_{\text{MN}}\rangle$ exhibits the same enhanced sensitivity as $|\Psi_{\text{MePe}}\rangle$, surpassing other probe states, regardless of the number of photons and nodes.

## II. EXPERIMENTAL DETAILS

### A. Experimental method

A distributed quantum sensing scheme for estimating the average of the two unknown phases using four-mode 2002 states is illustrated in Supplemental Figure 3, corresponding to Figure 2 of the main text. In this experiment, a continuous-wave laser with a central wavelength of 780.25 nm serves as the pump laser, initially polarized to $|H\rangle$. The polarization is adjusted to $|D\rangle = (|H\rangle + |V\rangle)/\sqrt{2}$ using a half wave plate (HWP) at an optical axis of $22.5^{\circ}$. Upon entering the dual-wavelength polarizing beam splitter (DWP), which operates at 780 nm and 1560 nm, the $|D\rangle$ polarization is split into horizontal ($|H\rangle$) and vertical ($|V\rangle$) polarizations. The $|H\rangle$ component propagates counterclockwise, while the $|V\rangle$ component propagates clockwise inside a Sagnac interferometer. The $|V\rangle$ polarization is then adjusted to $|H\rangle$ after passing through a dual wavelength HWP (DWH) that operates at both wavelengths. The counter-propagating beams probabilistically generate a pair of 1560 nm photons with orthogonal polarizations ($|H\rangle$ and $|V\rangle$) in a 10 mm-thick type-II periodically poled $KTiOPO_4$ (PPKTP) crystal with a 46.2 $\mu$m poling period via spontaneous parametric down conversion (SPDC).

After the DWP, the polarization Bell state $(|HV\rangle + e^{i\varphi}|VH\rangle)/\sqrt{2}$ is prepared, where $\varphi$ denotes a relative phase [1]. Finally, using a DWH, the Bell state is set to $|\Phi\rangle = (|HH\rangle + e^{i\varphi}|VV\rangle)/\sqrt{2}$. $|\Phi\rangle$ is then sent to a lateral beam

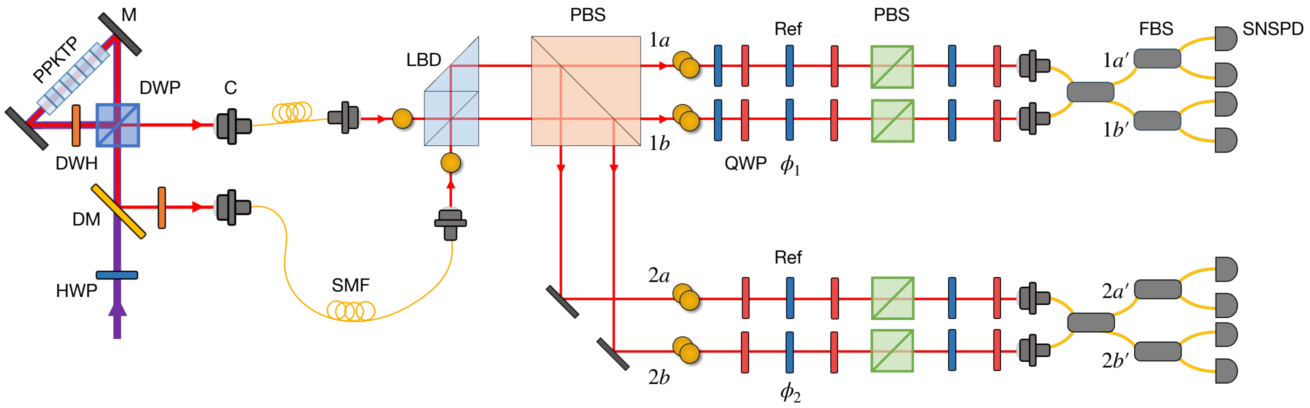


Supplemental Figure 3. **Experimental setup for implementing distributed quantum sensing scheme to estimate the average of the two phases using four-mode 2002 states.** HWP: half waveplate; DM: dichroic mirror; DWP: dual wavelength PBS; DWH: dual wavelength HWP; M: mirror; PPKTP: periodical poled KTiOPO; C: coupler; SMF: single mode fiber; LBD: lateral beam displacer; PBS: polarizing beam splitter; QWP: quarter waveplate; FBS: 50/50 fiber beam splitter, SNSPD: superconducting nanowire single-photon detector.

displacer (LBD) at each port, where the Hong-Ou-Mandel (HOM) effect occurs, resulting in two-photon interference. After passing through polarization beam splitters (PBS) and HWP set to 45°, we can prepare four-mode 2002 states, $|\Psi_4^2\rangle = (|20\rangle_1|00\rangle_2 + |02\rangle_1|00\rangle_2 + |00\rangle_1|20\rangle_2 + |00\rangle_1|02\rangle_2)/2$. The probe state then undergoes phase encoding using a combination of two QWPs with an optic axes at 45° and a HWP as shown in Supplemental Figure 3 [1]. After encoding two phases $\phi$, the probe state $|\Psi_4^2\rangle$ evolves into $\hat{U}(\phi)|\Psi_4^2\rangle$. Then, projective measurements were performed using 50/50 fiber beam splitters (FBSs) at each node and superconducting nanowire single-photon detectors (SNSPDs), functioning as PNDRs. We can then obtain the post-selected two-photon detection probabilities of $\{P_1^{11}, P_1^{20}, P_1^{02}, P_2^{11}, P_2^{20}, P_2^{02}\}$ with positive operator-valued measures (POVM) $\{\hat{\Pi}_l\} = \{|20\rangle\langle 20|_1, |11\rangle\langle 11|_1, |02\rangle\langle 02|_1, |20\rangle\langle 20|_2, |11\rangle\langle 11|_2, |02\rangle\langle 02|_2\}$, using Supplemental Eq. (7), as shown in the Figure 3(a) of the main text. The corresponding probabilities are as follows:

$$
\begin{aligned}
P_1^{11} &= \frac{1+\mathrm{V}_1^{11}\cos(2\phi_1)}{4},\; P_1^{20} = P_1^{02} = \frac{1-\mathrm{V}_1^{20(02)}\cos(2\phi_1)}{8},\\
P_2^{11} &= \frac{1+\mathrm{V}_2^{11}\cos(2\phi_2)}{4},\; P_2^{20} = P_2^{02} = \frac{1-\mathrm{V}_2^{20(02)}\cos(2\phi_2)}{8},
\end{aligned}
\tag{21}
$$

where $\mathrm{V}_j^{11}$ and $\mathrm{V}_j^{20(02)}$ denote the visibility for two-photon detection probabilities, and subscript $j$ denotes the node, i.e., $j = \{1, 2\}$.

We then calculate $\mathbf{F}_{\mathrm{C(exp)}}^{\mathrm{MN}}$ using Supplemental Eq. (21) with experimentally obtained visibilities as follows:

$$
\mathbf{F}_{\mathrm{C(exp)}} = \begin{pmatrix} 1.78 & 0 \\ 0 & 1.99 \end{pmatrix}. \tag{22}
$$

Using the Supplemental Eq. (22) with $\boldsymbol{\nu} = (1/2, 1/2)$, the experimentally obtained CRB is evaluated to be 1/3.76. The experimentally obtained shape of the standard deviation curve is calculated using $\Delta\phi = \sqrt{\boldsymbol{\nu}^T \mathbf{F}_{\mathrm{C}}^{-1} \boldsymbol{\nu}/\mu}$, which depends on the derivative of the probability functions with respect to phases. Around $\phi = \pi/2$, the slope of the probability functions becomes minimal, leading to a decrease in the Fisher inforamtion value and thus a divergence in the standard deviation as shown in Fig. 3(c) of the main text.

### B. Estimation error

The estimated phase $\phi_{\mathrm{est}}$ and its standard deviation $\Delta\phi_{\mathrm{est}}$ were determined using the standard bootstrapping method, applied to repeated measurements at the phase values we set [6]. In our experiments, we conducted 4,931 measurements, repeating the process 10 times. From these, we created 100 randomly selected groups from the 10 measured sets, and $\phi_{\mathrm{est}}$ and $\Delta\phi_{\mathrm{est}}$ were obtained using maximum likelihood estimation (MLE), as shown in Fig. 3(c) of the Main text. The error bars were calculated using $\delta(\Delta\phi) = \Delta\phi/\sqrt{2(s-1)}$, with $s = 100$ groups [2, 3].

[1] S. Hong, Y.-S. Kim, Y.-W. Cho, S.-W. Lee, H. Jung, S. Moon, S.-W. Han, and H.-T. Lim, Quantum enhanced multiple-phase estimation with multi-mode NOON states, Quantum enhanced multiple-phase estimation with multi-mode $N00N$ states, Nat. Commun. **12**, 1 (2021).

[2] L.-Z. Liu, Y.-Z. Zhang, Z.-D. Li, R. Zhang, X.-F. Yin, Y.-Y. Fei, L. Li, N.-L. Liu, F. Xu, Y.-A. Chen, and J.-W. Pan, Distributed quantum phase estimation with entangled photons, Nat. Photon. **15**, 137 (2021).

[3] S.-R. Zhao, Y.-Z. Zhang, W.-Z. Liu, J.-Y. Guan, W. Zhang, C.-L. Li, B. Bai, M.-H. Li, Y. Liu, L. You, J. Zhang, J. Fan, F. Xu, Q. Zhang, and J.-W. Pan, Field demonstration of distributed quantum sensing without post-selection, Phys. Rev. X **11**, 031009 (2021).

[4] J. P. Dowling. Quantum optical metrology — the lowdown on high-N00N states. Contemp. Phys. **49**, 125–143 (2008).

[5] M. Gessner, L. Pezzè, and A. Smerzi, Sensitivity Bounds for Multiparameter Quantum Metrology. Phys. Rev. Lett. **121**, 130503 (2018).

[6] S. Slussarenko, M. M. Weston, H. M. Chrzanowski, L. K. Shalm, V. B. Verma, S. W. Nam, and G. J. Pryde, Unconditional violation of the shot-noise limit in photonic quantum metrology. Nat. Photon. **11**, 700–703 (2017).
